# Supplementary material for: Stochastic excitation of internal gravity waves in rotating late F-type stars: A 3D simulation approach
Source: arXiv:2208.14759 source file (2022-08-31)
Supplement: Supplementary file 1 [file appendix_depth_map.tex]

\section{Power spectra radial evolution \label{appendix:power_spectrum_radial_evolution}}

\begin{figure*}[ht!]
    \centering
    \includegraphics[width=\textwidth]{figures/assembled_depth_map_l1_alt.pdf}
    \caption{Power spectrum for $\ell=1$, $E_1$, radial evolution in the F1a (\textit{top left}), F1b (\textit{top right}),  F3 (\textit{bottom left}), and F5 (\textit{bottom right}) cases. In each panel, the white line highlights the boundary of the mode resonant cavity.}
    \label{fig:depth_map_l1}
\end{figure*}

Complementary to the radial evolution of the $E_4$ power spectrum shown in Fig.~\ref{fig:depth_map_l4}, we present in this Appendix the $E_\ell$ power spectrum radial evolution for $\ell =1$, 2, 3, 5, 6, 7 and 8 in Fig.~\ref{fig:depth_map_l1}, \ref{fig:depth_map_l2}, \ref{fig:depth_map_l3}, \ref{fig:depth_map_l5}, \ref{fig:depth_map_l6}, \ref{fig:depth_map_l7}, and \ref{fig:depth_map_l8}, respectively. For the $E_1$ spectrum, the splitted structure of the modes is particularly visible for fast rotating cases. The rotational splittings are more difficult to distinguish for $\ell \geq 2$, in the co-rotational frame, $|\delta_{n \ell m}|$ decrease with increasing $\ell$ according to Eq.~\ref{eq:delta_nlm_corotational_frame} and \ref{eq:beta_nl}. As underlined in Sect.~\ref{sec:igw_spectrum}, the cutoff between g modes and progressive waves is located at decreasing period for increasing $\ell$. 

\begin{figure*}[ht!]
    \centering
    \includegraphics[width=\textwidth]{figures/assembled_depth_map_l2_alt.pdf}
    \caption{Power spectrum for $\ell=2$, $E_2$, radial evolution in the F1a (\textit{top left}), F1b (\textit{top right}),  F3 (\textit{bottom left}), and F5 (\textit{bottom right}) cases. In each panel, the white line highlights the boundary of the mode resonant cavity.}
    \label{fig:depth_map_l2}
\end{figure*}

\begin{figure*}[ht!]
    \centering
    \includegraphics[width=\textwidth]{figures/assembled_depth_map_l3_alt.pdf}
    \caption{Power spectrum for $\ell=3$, $E_3$, radial evolution in the F1a (\textit{top left}), F1b (\textit{top right}),  F3 (\textit{bottom left}), and F5 (\textit{bottom right}) cases. In each panel, the white line highlights the boundary of the mode resonant cavity.}
    \label{fig:depth_map_l3}
\end{figure*}

\begin{figure*}[ht!]
    \centering
    \includegraphics[width=\textwidth]{figures/assembled_depth_map_l5_alt.pdf}
    \caption{Power spectrum for $\ell=5$, $E_5$, radial evolution in the F1a (\textit{top left}), F1b (\textit{top right}),  F3 (\textit{bottom left}), and F5 (\textit{bottom right}) cases. In each panel, the white line highlights the boundary of the mode resonant cavity.}
    \label{fig:depth_map_l5}
\end{figure*}

\begin{figure*}[ht!]
    \centering
    \includegraphics[width=\textwidth]{figures/assembled_depth_map_l6_alt.pdf}
    \caption{Power spectrum for $\ell=6$, $E_6$, radial evolution in the F1a (\textit{top left}), F1b (\textit{top right}),  F3 (\textit{bottom left}), and F5 (\textit{bottom right}) cases. In each panel, the white line highlights the boundary of the mode resonant cavity.}
    \label{fig:depth_map_l6}
\end{figure*}

\begin{figure*}[ht!]
    \centering
    \includegraphics[width=\textwidth]{figures/assembled_depth_map_l7_alt.pdf}
    \caption{Power spectrum for $\ell=7$, $E_7$, radial evolution in the F1a (\textit{top left}), F1b (\textit{top right}),  F3 (\textit{bottom left}), and F5 (\textit{bottom right}) cases. In each panel, the white line highlights the boundary of the mode resonant cavity.}
    \label{fig:depth_map_l7}
\end{figure*}

\begin{figure*}[ht!]
    \centering
    \includegraphics[width=\textwidth]{figures/assembled_depth_map_l8_alt.pdf}
    \caption{Power spectrum for $\ell=8$, $E_8$, radial evolution in the F1a (\textit{top left}), F1b (\textit{top right}),  F3 (\textit{bottom left}), and F5 (\textit{bottom right}) cases. In each panel, the white line highlights the boundary of the mode resonant cavity.}
    \label{fig:depth_map_l8}
\end{figure*}
